# Supplementary material for: Cross-Inlining Binary Function Similarity Detection
Source: arXiv:2401.05739 source file (2024-01-11)
Supplement: Supplementary file 1 [file 8-appendix.tex]

\section{Appendix}

% Please add the following required packages to your document preamble:
% \usepackage{multirow}
\begin{table*}[b]
	\caption{Effectiveness of existing works according to the threshold}
	\vspace{-10pt}
	\scalebox{0.8}{
\begin{tabular}{c|c|c|ccccccccccccccccccc}
	\hline
	\multirow{2}{*}{Method}  & \multirow{2}{*}{Patterns}  & \multirow{2}{*}{Metrics} & \multicolumn{19}{c}{Threshold}                                                                                                                                                                                                                                                                                                                                                                                                                                                                                                                                                    \\ \cline{4-22} 
	&                            &                          & \multicolumn{1}{c|}{0.05}          & \multicolumn{1}{c|}{0.1}           & \multicolumn{1}{c|}{0.15}          & \multicolumn{1}{c|}{0.2}           & \multicolumn{1}{c|}{0.25}          & \multicolumn{1}{c|}{0.3}  & \multicolumn{1}{c|}{0.35} & \multicolumn{1}{c|}{0.4}  & \multicolumn{1}{c|}{0.45} & \multicolumn{1}{c|}{0.5}  & \multicolumn{1}{c|}{0.55} & \multicolumn{1}{c|}{0.6}           & \multicolumn{1}{c|}{0.65} & \multicolumn{1}{c|}{0.7}  & \multicolumn{1}{c|}{0.75} & \multicolumn{1}{c|}{0.8}  & \multicolumn{1}{c|}{0.85} & \multicolumn{1}{c|}{0.9}  & 0.95 \\ \hline
	\multirow{12}{*}{Gemini} & \multirow{4}{*}{Inlinined} & Accuracy                 & \multicolumn{1}{c|}{0.50}          & \multicolumn{1}{c|}{0.50}          & \multicolumn{1}{c|}{0.50}          & \multicolumn{1}{c|}{\textbf{0.50}} & \multicolumn{1}{c|}{0.51}          & \multicolumn{1}{c|}{0.51} & \multicolumn{1}{c|}{0.53} & \multicolumn{1}{c|}{0.55} & \multicolumn{1}{c|}{0.57} & \multicolumn{1}{c|}{0.57} & \multicolumn{1}{c|}{0.57} & \multicolumn{1}{c|}{0.57}          & \multicolumn{1}{c|}{0.57} & \multicolumn{1}{c|}{0.56} & \multicolumn{1}{c|}{0.56} & \multicolumn{1}{c|}{0.55} & \multicolumn{1}{c|}{0.54} & \multicolumn{1}{c|}{0.53} & 0.51 \\ \cline{3-22} 
	&                            & Precision                & \multicolumn{1}{c|}{0.50}          & \multicolumn{1}{c|}{0.50}          & \multicolumn{1}{c|}{0.50}          & \multicolumn{1}{c|}{0.50}          & \multicolumn{1}{c|}{0.50}          & \multicolumn{1}{c|}{0.51} & \multicolumn{1}{c|}{0.52} & \multicolumn{1}{c|}{0.53} & \multicolumn{1}{c|}{0.56} & \multicolumn{1}{c|}{0.58} & \multicolumn{1}{c|}{0.61} & \multicolumn{1}{c|}{0.63}          & \multicolumn{1}{c|}{0.66} & \multicolumn{1}{c|}{0.69} & \multicolumn{1}{c|}{0.72} & \multicolumn{1}{c|}{0.74} & \multicolumn{1}{c|}{0.77} & \multicolumn{1}{c|}{0.81} & 0.84 \\ \cline{3-22} 
	&                            & Recall                   & \multicolumn{1}{c|}{1.00}          & \multicolumn{1}{c|}{1.00}          & \multicolumn{1}{c|}{1.00}          & \multicolumn{1}{c|}{0.99}          & \multicolumn{1}{c|}{0.97}          & \multicolumn{1}{c|}{0.93} & \multicolumn{1}{c|}{0.87} & \multicolumn{1}{c|}{0.78} & \multicolumn{1}{c|}{0.65} & \multicolumn{1}{c|}{0.52} & \multicolumn{1}{c|}{0.42} & \multicolumn{1}{c|}{0.34}          & \multicolumn{1}{c|}{0.28} & \multicolumn{1}{c|}{0.23} & \multicolumn{1}{c|}{0.19} & \multicolumn{1}{c|}{0.14} & \multicolumn{1}{c|}{0.10} & \multicolumn{1}{c|}{0.07} & 0.03 \\ \cline{3-22} 
	&                            & F1                       & \multicolumn{1}{c|}{0.67}          & \multicolumn{1}{c|}{0.67}          & \multicolumn{1}{c|}{\textbf{0.67}} & \multicolumn{1}{c|}{\textbf{0.67}} & \multicolumn{1}{c|}{0.66}          & \multicolumn{1}{c|}{0.66} & \multicolumn{1}{c|}{0.65} & \multicolumn{1}{c|}{0.64} & \multicolumn{1}{c|}{0.60} & \multicolumn{1}{c|}{0.55} & \multicolumn{1}{c|}{0.49} & \multicolumn{1}{c|}{0.44}          & \multicolumn{1}{c|}{0.40} & \multicolumn{1}{c|}{0.35} & \multicolumn{1}{c|}{0.30} & \multicolumn{1}{c|}{0.24} & \multicolumn{1}{c|}{0.18} & \multicolumn{1}{c|}{0.13} & 0.06 \\ \cline{2-22} 
	& \multirow{4}{*}{Inlining}  & Accuracy                 & \multicolumn{1}{c|}{0.50}          & \multicolumn{1}{c|}{0.50}          & \multicolumn{1}{c|}{0.50}          & \multicolumn{1}{c|}{0.51}          & \multicolumn{1}{c|}{0.51}          & \multicolumn{1}{c|}{0.53} & \multicolumn{1}{c|}{0.56} & \multicolumn{1}{c|}{0.60} & \multicolumn{1}{c|}{0.64} & \multicolumn{1}{c|}{0.67} & \multicolumn{1}{c|}{0.70} & \multicolumn{1}{c|}{0.71}          & \multicolumn{1}{c|}{0.73} & \multicolumn{1}{c|}{0.73} & \multicolumn{1}{c|}{0.73} & \multicolumn{1}{c|}{0.72} & \multicolumn{1}{c|}{0.70} & \multicolumn{1}{c|}{0.67} & 0.62 \\ \cline{3-22} 
	&                            & Precision                & \multicolumn{1}{c|}{0.50}          & \multicolumn{1}{c|}{0.50}          & \multicolumn{1}{c|}{0.50}          & \multicolumn{1}{c|}{0.50}          & \multicolumn{1}{c|}{0.51}          & \multicolumn{1}{c|}{0.52} & \multicolumn{1}{c|}{0.54} & \multicolumn{1}{c|}{0.56} & \multicolumn{1}{c|}{0.59} & \multicolumn{1}{c|}{0.63} & \multicolumn{1}{c|}{0.66} & \multicolumn{1}{c|}{0.69}          & \multicolumn{1}{c|}{0.72} & \multicolumn{1}{c|}{0.76} & \multicolumn{1}{c|}{0.79} & \multicolumn{1}{c|}{0.83} & \multicolumn{1}{c|}{0.86} & \multicolumn{1}{c|}{0.90} & 0.95 \\ \cline{3-22} 
	&                            & Recall                   & \multicolumn{1}{c|}{1.00}          & \multicolumn{1}{c|}{1.00}          & \multicolumn{1}{c|}{1.00}          & \multicolumn{1}{c|}{\textbf{1.00}} & \multicolumn{1}{c|}{0.99}          & \multicolumn{1}{c|}{0.99} & \multicolumn{1}{c|}{0.97} & \multicolumn{1}{c|}{0.94} & \multicolumn{1}{c|}{0.89} & \multicolumn{1}{c|}{0.85} & \multicolumn{1}{c|}{0.81} & \multicolumn{1}{c|}{0.77}          & \multicolumn{1}{c|}{0.73} & \multicolumn{1}{c|}{0.68} & \multicolumn{1}{c|}{0.63} & \multicolumn{1}{c|}{0.57} & \multicolumn{1}{c|}{0.48} & \multicolumn{1}{c|}{0.39} & 0.26 \\ \cline{3-22} 
	&                            & F1                       & \multicolumn{1}{c|}{0.67}          & \multicolumn{1}{c|}{0.67}          & \multicolumn{1}{c|}{0.67}          & \multicolumn{1}{c|}{0.67}          & \multicolumn{1}{c|}{0.67}          & \multicolumn{1}{c|}{0.68} & \multicolumn{1}{c|}{0.69} & \multicolumn{1}{c|}{0.70} & \multicolumn{1}{c|}{0.71} & \multicolumn{1}{c|}{0.72} & \multicolumn{1}{c|}{0.73} & \multicolumn{1}{c|}{\textbf{0.73}} & \multicolumn{1}{c|}{0.73} & \multicolumn{1}{c|}{0.71} & \multicolumn{1}{c|}{0.70} & \multicolumn{1}{c|}{0.67} & \multicolumn{1}{c|}{0.62} & \multicolumn{1}{c|}{0.54} & 0.41 \\ \cline{2-22} 
	& \multirow{4}{*}{Recursive} & Accuracy                 & \multicolumn{1}{c|}{0.50}          & \multicolumn{1}{c|}{0.50}          & \multicolumn{1}{c|}{0.50}          & \multicolumn{1}{c|}{0.50}          & \multicolumn{1}{c|}{0.50}          & \multicolumn{1}{c|}{0.51} & \multicolumn{1}{c|}{0.52} & \multicolumn{1}{c|}{0.53} & \multicolumn{1}{c|}{0.55} & \multicolumn{1}{c|}{0.55} & \multicolumn{1}{c|}{0.56} & \multicolumn{1}{c|}{0.56}          & \multicolumn{1}{c|}{0.56} & \multicolumn{1}{c|}{0.56} & \multicolumn{1}{c|}{0.54} & \multicolumn{1}{c|}{0.53} & \multicolumn{1}{c|}{0.52} & \multicolumn{1}{c|}{0.51} & 0.51 \\ \cline{3-22} 
	&                            & Precision                & \multicolumn{1}{c|}{0.50}          & \multicolumn{1}{c|}{0.50}          & \multicolumn{1}{c|}{0.50}          & \multicolumn{1}{c|}{0.50}          & \multicolumn{1}{c|}{0.50}          & \multicolumn{1}{c|}{0.50} & \multicolumn{1}{c|}{0.51} & \multicolumn{1}{c|}{0.52} & \multicolumn{1}{c|}{0.54} & \multicolumn{1}{c|}{0.56} & \multicolumn{1}{c|}{0.58} & \multicolumn{1}{c|}{0.60}          & \multicolumn{1}{c|}{0.62} & \multicolumn{1}{c|}{0.63} & \multicolumn{1}{c|}{0.64} & \multicolumn{1}{c|}{0.64} & \multicolumn{1}{c|}{0.64} & \multicolumn{1}{c|}{0.61} & 0.63 \\ \cline{3-22} 
	&                            & Recall                   & \multicolumn{1}{c|}{1.00}          & \multicolumn{1}{c|}{1.00}          & \multicolumn{1}{c|}{1.00}          & \multicolumn{1}{c|}{0.99}          & \multicolumn{1}{c|}{0.97}          & \multicolumn{1}{c|}{0.93} & \multicolumn{1}{c|}{0.87} & \multicolumn{1}{c|}{0.75} & \multicolumn{1}{c|}{0.63} & \multicolumn{1}{c|}{0.51} & \multicolumn{1}{c|}{0.44} & \multicolumn{1}{c|}{0.38}          & \multicolumn{1}{c|}{0.32} & \multicolumn{1}{c|}{0.27} & \multicolumn{1}{c|}{0.21} & \multicolumn{1}{c|}{0.15} & \multicolumn{1}{c|}{0.10} & \multicolumn{1}{c|}{0.06} & 0.03 \\ \cline{3-22} 
	&                            & F1                       & \multicolumn{1}{c|}{0.67}          & \multicolumn{1}{c|}{\textbf{0.67}} & \multicolumn{1}{c|}{0.67}          & \multicolumn{1}{c|}{0.66}          & \multicolumn{1}{c|}{0.66}          & \multicolumn{1}{c|}{0.65} & \multicolumn{1}{c|}{0.65} & \multicolumn{1}{c|}{0.62} & \multicolumn{1}{c|}{0.58} & \multicolumn{1}{c|}{0.53} & \multicolumn{1}{c|}{0.50} & \multicolumn{1}{c|}{0.47}          & \multicolumn{1}{c|}{0.42} & \multicolumn{1}{c|}{0.38} & \multicolumn{1}{c|}{0.31} & \multicolumn{1}{c|}{0.25} & \multicolumn{1}{c|}{0.18} & \multicolumn{1}{c|}{0.10} & 0.05 \\ \hline
	\multirow{12}{*}{Safe}   & \multirow{4}{*}{Inlinined} & Accuracy                 & \multicolumn{1}{c|}{0.53}          & \multicolumn{1}{c|}{0.53}          & \multicolumn{1}{c|}{0.53}          & \multicolumn{1}{c|}{0.53}          & \multicolumn{1}{c|}{0.52}          & \multicolumn{1}{c|}{0.52} & \multicolumn{1}{c|}{0.52} & \multicolumn{1}{c|}{0.52} & \multicolumn{1}{c|}{0.52} & \multicolumn{1}{c|}{0.52} & \multicolumn{1}{c|}{0.52} & \multicolumn{1}{c|}{0.52}          & \multicolumn{1}{c|}{0.52} & \multicolumn{1}{c|}{0.52} & \multicolumn{1}{c|}{0.51} & \multicolumn{1}{c|}{0.51} & \multicolumn{1}{c|}{0.51} & \multicolumn{1}{c|}{0.51} & 0.51 \\ \cline{3-22} 
	&                            & Precision                & \multicolumn{1}{c|}{0.53}          & \multicolumn{1}{c|}{0.54}          & \multicolumn{1}{c|}{0.54}          & \multicolumn{1}{c|}{0.55}          & \multicolumn{1}{c|}{0.55}          & \multicolumn{1}{c|}{0.55} & \multicolumn{1}{c|}{0.55} & \multicolumn{1}{c|}{0.56} & \multicolumn{1}{c|}{0.56} & \multicolumn{1}{c|}{0.57} & \multicolumn{1}{c|}{0.57} & \multicolumn{1}{c|}{0.57}          & \multicolumn{1}{c|}{0.58} & \multicolumn{1}{c|}{0.58} & \multicolumn{1}{c|}{0.59} & \multicolumn{1}{c|}{0.60} & \multicolumn{1}{c|}{0.61} & \multicolumn{1}{c|}{0.64} & 0.68 \\ \cline{3-22} 
	&                            & Recall                   & \multicolumn{1}{c|}{0.53}          & \multicolumn{1}{c|}{0.43}          & \multicolumn{1}{c|}{0.36}          & \multicolumn{1}{c|}{0.31}          & \multicolumn{1}{c|}{0.28}          & \multicolumn{1}{c|}{0.25} & \multicolumn{1}{c|}{0.23} & \multicolumn{1}{c|}{0.21} & \multicolumn{1}{c|}{0.19} & \multicolumn{1}{c|}{0.17} & \multicolumn{1}{c|}{0.16} & \multicolumn{1}{c|}{0.14}          & \multicolumn{1}{c|}{0.13} & \multicolumn{1}{c|}{0.11} & \multicolumn{1}{c|}{0.09} & \multicolumn{1}{c|}{0.07} & \multicolumn{1}{c|}{0.06} & \multicolumn{1}{c|}{0.04} & 0.03 \\ \cline{3-22} 
	&                            & F1                       & \multicolumn{1}{c|}{\textbf{0.53}} & \multicolumn{1}{c|}{0.47}          & \multicolumn{1}{c|}{0.43}          & \multicolumn{1}{c|}{0.40}          & \multicolumn{1}{c|}{0.37}          & \multicolumn{1}{c|}{0.34} & \multicolumn{1}{c|}{0.33} & \multicolumn{1}{c|}{0.30} & \multicolumn{1}{c|}{0.28} & \multicolumn{1}{c|}{0.27} & \multicolumn{1}{c|}{0.25} & \multicolumn{1}{c|}{0.23}          & \multicolumn{1}{c|}{0.21} & \multicolumn{1}{c|}{0.18} & \multicolumn{1}{c|}{0.16} & \multicolumn{1}{c|}{0.13} & \multicolumn{1}{c|}{0.10} & \multicolumn{1}{c|}{0.08} & 0.05 \\ \cline{2-22} 
	& \multirow{4}{*}{Inlining}  & Accuracy                 & \multicolumn{1}{c|}{0.60}          & \multicolumn{1}{c|}{0.62}          & \multicolumn{1}{c|}{0.64}          & \multicolumn{1}{c|}{0.65}          & \multicolumn{1}{c|}{0.67}          & \multicolumn{1}{c|}{0.67} & \multicolumn{1}{c|}{0.68} & \multicolumn{1}{c|}{0.68} & \multicolumn{1}{c|}{0.68} & \multicolumn{1}{c|}{0.68} & \multicolumn{1}{c|}{0.68} & \multicolumn{1}{c|}{0.68}          & \multicolumn{1}{c|}{0.68} & \multicolumn{1}{c|}{0.67} & \multicolumn{1}{c|}{0.67} & \multicolumn{1}{c|}{0.66} & \multicolumn{1}{c|}{0.64} & \multicolumn{1}{c|}{0.61} & 0.58 \\ \cline{3-22} 
	&                            & Precision                & \multicolumn{1}{c|}{0.56}          & \multicolumn{1}{c|}{0.58}          & \multicolumn{1}{c|}{0.60}          & \multicolumn{1}{c|}{0.61}          & \multicolumn{1}{c|}{0.62}          & \multicolumn{1}{c|}{0.63} & \multicolumn{1}{c|}{0.64} & \multicolumn{1}{c|}{0.65} & \multicolumn{1}{c|}{0.66} & \multicolumn{1}{c|}{0.67} & \multicolumn{1}{c|}{0.68} & \multicolumn{1}{c|}{0.69}          & \multicolumn{1}{c|}{0.70} & \multicolumn{1}{c|}{0.71} & \multicolumn{1}{c|}{0.73} & \multicolumn{1}{c|}{0.74} & \multicolumn{1}{c|}{0.76} & \multicolumn{1}{c|}{0.79} & 0.81 \\ \cline{3-22} 
	&                            & Recall                   & \multicolumn{1}{c|}{0.94}          & \multicolumn{1}{c|}{0.92}          & \multicolumn{1}{c|}{0.89}          & \multicolumn{1}{c|}{0.87}          & \multicolumn{1}{c|}{0.85}          & \multicolumn{1}{c|}{0.83} & \multicolumn{1}{c|}{0.81} & \multicolumn{1}{c|}{0.79} & \multicolumn{1}{c|}{0.76} & \multicolumn{1}{c|}{0.73} & \multicolumn{1}{c|}{0.70} & \multicolumn{1}{c|}{0.66}          & \multicolumn{1}{c|}{0.63} & \multicolumn{1}{c|}{0.58} & \multicolumn{1}{c|}{0.53} & \multicolumn{1}{c|}{0.47} & \multicolumn{1}{c|}{0.40} & \multicolumn{1}{c|}{0.31} & 0.20 \\ \cline{3-22} 
	&                            & F1                       & \multicolumn{1}{c|}{0.70}          & \multicolumn{1}{c|}{0.71}          & \multicolumn{1}{c|}{0.71}          & \multicolumn{1}{c|}{0.72}          & \multicolumn{1}{c|}{\textbf{0.72}} & \multicolumn{1}{c|}{0.72} & \multicolumn{1}{c|}{0.72} & \multicolumn{1}{c|}{0.71} & \multicolumn{1}{c|}{0.70} & \multicolumn{1}{c|}{0.70} & \multicolumn{1}{c|}{0.69} & \multicolumn{1}{c|}{0.68}          & \multicolumn{1}{c|}{0.66} & \multicolumn{1}{c|}{0.64} & \multicolumn{1}{c|}{0.61} & \multicolumn{1}{c|}{0.58} & \multicolumn{1}{c|}{0.53} & \multicolumn{1}{c|}{0.44} & 0.32 \\ \cline{2-22} 
	& \multirow{4}{*}{Recursive} & Accuracy                 & \multicolumn{1}{c|}{0.52}          & \multicolumn{1}{c|}{0.53}          & \multicolumn{1}{c|}{0.53}          & \multicolumn{1}{c|}{0.54}          & \multicolumn{1}{c|}{0.54}          & \multicolumn{1}{c|}{0.54} & \multicolumn{1}{c|}{0.54} & \multicolumn{1}{c|}{0.54} & \multicolumn{1}{c|}{0.54} & \multicolumn{1}{c|}{0.53} & \multicolumn{1}{c|}{0.53} & \multicolumn{1}{c|}{0.53}          & \multicolumn{1}{c|}{0.53} & \multicolumn{1}{c|}{0.53} & \multicolumn{1}{c|}{0.53} & \multicolumn{1}{c|}{0.52} & \multicolumn{1}{c|}{0.52} & \multicolumn{1}{c|}{0.52} & 0.51 \\ \cline{3-22} 
	&                            & Precision                & \multicolumn{1}{c|}{0.52}          & \multicolumn{1}{c|}{0.52}          & \multicolumn{1}{c|}{0.53}          & \multicolumn{1}{c|}{0.54}          & \multicolumn{1}{c|}{0.54}          & \multicolumn{1}{c|}{0.55} & \multicolumn{1}{c|}{0.55} & \multicolumn{1}{c|}{0.55} & \multicolumn{1}{c|}{0.56} & \multicolumn{1}{c|}{0.55} & \multicolumn{1}{c|}{0.56} & \multicolumn{1}{c|}{0.56}          & \multicolumn{1}{c|}{0.56} & \multicolumn{1}{c|}{0.56} & \multicolumn{1}{c|}{0.57} & \multicolumn{1}{c|}{0.57} & \multicolumn{1}{c|}{0.58} & \multicolumn{1}{c|}{0.60} & 0.62 \\ \cline{3-22} 
	&                            & Recall                   & \multicolumn{1}{c|}{0.71}          & \multicolumn{1}{c|}{0.63}          & \multicolumn{1}{c|}{0.57}          & \multicolumn{1}{c|}{0.53}          & \multicolumn{1}{c|}{0.50}          & \multicolumn{1}{c|}{0.47} & \multicolumn{1}{c|}{0.44} & \multicolumn{1}{c|}{0.41} & \multicolumn{1}{c|}{0.38} & \multicolumn{1}{c|}{0.35} & \multicolumn{1}{c|}{0.32} & \multicolumn{1}{c|}{0.30}          & \multicolumn{1}{c|}{0.27} & \multicolumn{1}{c|}{0.25} & \multicolumn{1}{c|}{0.22} & \multicolumn{1}{c|}{0.19} & \multicolumn{1}{c|}{0.15} & \multicolumn{1}{c|}{0.11} & 0.07 \\ \cline{3-22} 
	&                            & F1                       & \multicolumn{1}{c|}{\textbf{0.60}} & \multicolumn{1}{c|}{0.57}          & \multicolumn{1}{c|}{0.55}          & \multicolumn{1}{c|}{0.53}          & \multicolumn{1}{c|}{0.52}          & \multicolumn{1}{c|}{0.50} & \multicolumn{1}{c|}{0.49} & \multicolumn{1}{c|}{0.47} & \multicolumn{1}{c|}{0.45} & \multicolumn{1}{c|}{0.43} & \multicolumn{1}{c|}{0.41} & \multicolumn{1}{c|}{0.39}          & \multicolumn{1}{c|}{0.37} & \multicolumn{1}{c|}{0.34} & \multicolumn{1}{c|}{0.32} & \multicolumn{1}{c|}{0.28} & \multicolumn{1}{c|}{0.24} & \multicolumn{1}{c|}{0.19} & 0.13 \\ \hline
	\multirow{12}{*}{GMN}    & \multirow{4}{*}{Inlinined} & Accuracy                 & \multicolumn{1}{c|}{0.56}          & \multicolumn{1}{c|}{0.55}          & \multicolumn{1}{c|}{0.55}          & \multicolumn{1}{c|}{0.55}          & \multicolumn{1}{c|}{0.55}          & \multicolumn{1}{c|}{0.55} & \multicolumn{1}{c|}{0.55} & \multicolumn{1}{c|}{0.54} & \multicolumn{1}{c|}{0.54} & \multicolumn{1}{c|}{0.50} & \multicolumn{1}{c|}{0.50} & \multicolumn{1}{c|}{0.50}          & \multicolumn{1}{c|}{0.50} & \multicolumn{1}{c|}{0.50} & \multicolumn{1}{c|}{0.50} & \multicolumn{1}{c|}{0.50} & \multicolumn{1}{c|}{0.50} & \multicolumn{1}{c|}{0.50} & 0.50 \\ \cline{3-22} 
	&                            & Precision                & \multicolumn{1}{c|}{0.56}          & \multicolumn{1}{c|}{0.56}          & \multicolumn{1}{c|}{0.56}          & \multicolumn{1}{c|}{0.57}          & \multicolumn{1}{c|}{0.58}          & \multicolumn{1}{c|}{0.58} & \multicolumn{1}{c|}{0.60} & \multicolumn{1}{c|}{0.62} & \multicolumn{1}{c|}{0.67} & \multicolumn{1}{c|}{0.00} & \multicolumn{1}{c|}{0.00} & \multicolumn{1}{c|}{0.00}          & \multicolumn{1}{c|}{0.00} & \multicolumn{1}{c|}{0.00} & \multicolumn{1}{c|}{0.00} & \multicolumn{1}{c|}{0.00} & \multicolumn{1}{c|}{0.00} & \multicolumn{1}{c|}{0.00} & 0.00 \\ \cline{3-22} 
	&                            & Recall                   & \multicolumn{1}{c|}{0.56}          & \multicolumn{1}{c|}{0.52}          & \multicolumn{1}{c|}{0.48}          & \multicolumn{1}{c|}{0.43}          & \multicolumn{1}{c|}{0.39}          & \multicolumn{1}{c|}{0.33} & \multicolumn{1}{c|}{0.28} & \multicolumn{1}{c|}{0.22} & \multicolumn{1}{c|}{0.14} & \multicolumn{1}{c|}{0.00} & \multicolumn{1}{c|}{0.00} & \multicolumn{1}{c|}{0.00}          & \multicolumn{1}{c|}{0.00} & \multicolumn{1}{c|}{0.00} & \multicolumn{1}{c|}{0.00} & \multicolumn{1}{c|}{0.00} & \multicolumn{1}{c|}{0.00} & \multicolumn{1}{c|}{0.00} & 0.00 \\ \cline{3-22} 
	&                            & F1                       & \multicolumn{1}{c|}{\textbf{0.56}} & \multicolumn{1}{c|}{0.54}          & \multicolumn{1}{c|}{0.52}          & \multicolumn{1}{c|}{0.49}          & \multicolumn{1}{c|}{0.46}          & \multicolumn{1}{c|}{0.43} & \multicolumn{1}{c|}{0.38} & \multicolumn{1}{c|}{0.33} & \multicolumn{1}{c|}{0.24} & \multicolumn{1}{c|}{0.00} & \multicolumn{1}{c|}{0.00} & \multicolumn{1}{c|}{0.00}          & \multicolumn{1}{c|}{0.00} & \multicolumn{1}{c|}{0.00} & \multicolumn{1}{c|}{0.00} & \multicolumn{1}{c|}{0.00} & \multicolumn{1}{c|}{0.00} & \multicolumn{1}{c|}{0.00} & 0.00 \\ \cline{2-22} 
	& \multirow{4}{*}{Inlining}  & Accuracy                 & \multicolumn{1}{c|}{0.69}          & \multicolumn{1}{c|}{0.70}          & \multicolumn{1}{c|}{0.71}          & \multicolumn{1}{c|}{0.73}          & \multicolumn{1}{c|}{0.74}          & \multicolumn{1}{c|}{0.75} & \multicolumn{1}{c|}{0.75} & \multicolumn{1}{c|}{0.75} & \multicolumn{1}{c|}{0.73} & \multicolumn{1}{c|}{0.50} & \multicolumn{1}{c|}{0.50} & \multicolumn{1}{c|}{0.50}          & \multicolumn{1}{c|}{0.50} & \multicolumn{1}{c|}{0.50} & \multicolumn{1}{c|}{0.50} & \multicolumn{1}{c|}{0.50} & \multicolumn{1}{c|}{0.50} & \multicolumn{1}{c|}{0.50} & 0.50 \\ \cline{3-22} 
	&                            & Precision                & \multicolumn{1}{c|}{0.64}          & \multicolumn{1}{c|}{0.65}          & \multicolumn{1}{c|}{0.67}          & \multicolumn{1}{c|}{0.69}          & \multicolumn{1}{c|}{0.71}          & \multicolumn{1}{c|}{0.74} & \multicolumn{1}{c|}{0.77} & \multicolumn{1}{c|}{0.81} & \multicolumn{1}{c|}{0.88} & \multicolumn{1}{c|}{1.00} & \multicolumn{1}{c|}{0.00} & \multicolumn{1}{c|}{0.00}          & \multicolumn{1}{c|}{0.00} & \multicolumn{1}{c|}{0.00} & \multicolumn{1}{c|}{0.00} & \multicolumn{1}{c|}{0.00} & \multicolumn{1}{c|}{0.00} & \multicolumn{1}{c|}{0.00} & 0.00 \\ \cline{3-22} 
	&                            & Recall                   & \multicolumn{1}{c|}{0.88}          & \multicolumn{1}{c|}{0.87}          & \multicolumn{1}{c|}{0.85}          & \multicolumn{1}{c|}{0.83}          & \multicolumn{1}{c|}{0.80}          & \multicolumn{1}{c|}{0.76} & \multicolumn{1}{c|}{0.72} & \multicolumn{1}{c|}{0.65} & \multicolumn{1}{c|}{0.54} & \multicolumn{1}{c|}{0.00} & \multicolumn{1}{c|}{0.00} & \multicolumn{1}{c|}{0.00}          & \multicolumn{1}{c|}{0.00} & \multicolumn{1}{c|}{0.00} & \multicolumn{1}{c|}{0.00} & \multicolumn{1}{c|}{0.00} & \multicolumn{1}{c|}{0.00} & \multicolumn{1}{c|}{0.00} & 0.00 \\ \cline{3-22} 
	&                            & F1                       & \multicolumn{1}{c|}{0.74}          & \multicolumn{1}{c|}{0.75}          & \multicolumn{1}{c|}{0.75}          & \multicolumn{1}{c|}{0.75}          & \multicolumn{1}{c|}{\textbf{0.75}} & \multicolumn{1}{c|}{0.75} & \multicolumn{1}{c|}{0.74} & \multicolumn{1}{c|}{0.72} & \multicolumn{1}{c|}{0.67} & \multicolumn{1}{c|}{0.00} & \multicolumn{1}{c|}{0.00} & \multicolumn{1}{c|}{0.00}          & \multicolumn{1}{c|}{0.00} & \multicolumn{1}{c|}{0.00} & \multicolumn{1}{c|}{0.00} & \multicolumn{1}{c|}{0.00} & \multicolumn{1}{c|}{0.00} & \multicolumn{1}{c|}{0.00} & 0.00 \\ \cline{2-22} 
	& \multirow{4}{*}{Recursive} & Accuracy                 & \multicolumn{1}{c|}{0.57}          & \multicolumn{1}{c|}{0.57}          & \multicolumn{1}{c|}{0.58}          & \multicolumn{1}{c|}{0.58}          & \multicolumn{1}{c|}{0.58}          & \multicolumn{1}{c|}{0.57} & \multicolumn{1}{c|}{0.56} & \multicolumn{1}{c|}{0.56} & \multicolumn{1}{c|}{0.55} & \multicolumn{1}{c|}{0.50} & \multicolumn{1}{c|}{0.50} & \multicolumn{1}{c|}{0.50}          & \multicolumn{1}{c|}{0.50} & \multicolumn{1}{c|}{0.50} & \multicolumn{1}{c|}{0.50} & \multicolumn{1}{c|}{0.50} & \multicolumn{1}{c|}{0.50} & \multicolumn{1}{c|}{0.50} & 0.50 \\ \cline{3-22} 
	&                            & Precision                & \multicolumn{1}{c|}{0.57}          & \multicolumn{1}{c|}{0.58}          & \multicolumn{1}{c|}{0.59}          & \multicolumn{1}{c|}{0.60}          & \multicolumn{1}{c|}{0.61}          & \multicolumn{1}{c|}{0.62} & \multicolumn{1}{c|}{0.64} & \multicolumn{1}{c|}{0.67} & \multicolumn{1}{c|}{0.72} & \multicolumn{1}{c|}{0.00} & \multicolumn{1}{c|}{0.00} & \multicolumn{1}{c|}{0.00}          & \multicolumn{1}{c|}{0.00} & \multicolumn{1}{c|}{0.00} & \multicolumn{1}{c|}{0.00} & \multicolumn{1}{c|}{0.00} & \multicolumn{1}{c|}{0.00} & \multicolumn{1}{c|}{0.00} & 0.00 \\ \cline{3-22} 
	&                            & Recall                   & \multicolumn{1}{c|}{0.57}          & \multicolumn{1}{c|}{0.53}          & \multicolumn{1}{c|}{0.50}          & \multicolumn{1}{c|}{0.46}          & \multicolumn{1}{c|}{0.41}          & \multicolumn{1}{c|}{0.35} & \multicolumn{1}{c|}{0.30} & \multicolumn{1}{c|}{0.24} & \multicolumn{1}{c|}{0.16} & \multicolumn{1}{c|}{0.00} & \multicolumn{1}{c|}{0.00} & \multicolumn{1}{c|}{0.00}          & \multicolumn{1}{c|}{0.00} & \multicolumn{1}{c|}{0.00} & \multicolumn{1}{c|}{0.00} & \multicolumn{1}{c|}{0.00} & \multicolumn{1}{c|}{0.00} & \multicolumn{1}{c|}{0.00} & 0.00 \\ \cline{3-22} 
	&                            & F1                       & \multicolumn{1}{c|}{\textbf{0.57}} & \multicolumn{1}{c|}{0.56}          & \multicolumn{1}{c|}{0.54}          & \multicolumn{1}{c|}{0.52}          & \multicolumn{1}{c|}{0.49}          & \multicolumn{1}{c|}{0.45} & \multicolumn{1}{c|}{0.40} & \multicolumn{1}{c|}{0.36} & \multicolumn{1}{c|}{0.26} & \multicolumn{1}{c|}{0.00} & \multicolumn{1}{c|}{0.00} & \multicolumn{1}{c|}{0.00}          & \multicolumn{1}{c|}{0.00} & \multicolumn{1}{c|}{0.00} & \multicolumn{1}{c|}{0.00} & \multicolumn{1}{c|}{0.00} & \multicolumn{1}{c|}{0.00} & \multicolumn{1}{c|}{0.00} & 0.00 \\ \hline
\end{tabular}
	}
\end{table*}
